# Supplementary material for: A Neural Hierarchical-Matrix Preconditioner for Real-Time GPU Solves
Source: arXiv:2605.13343 source file (2026-09-24)
Supplement: Supplementary file 1 [file supplementary-arxiv.tex]

% Supplementary material for "Hierarchical Transformer Preconditioning for Interactive Physics Simulation"
% arXiv preprint — uses ACM acmtog template for layout (fonts, margins, columns)
% but without TOG journal metadata (conference name, copyright, submission IDs)
% per SIGGRAPH Asia 2026 anonymity policy.
\documentclass[acmtog]{acmart}

\citestyle{acmauthoryear}
\setcopyright{none}
\settopmatter{printacmref=false, printccs=false, printfolios=true}
\renewcommand\footnotetextcopyrightpermission[1]{}
% Suppress the acmtog running footer (Vol./No./Article/Publication date)
\AtBeginDocument{\pagestyle{plain}}

\usepackage{amsmath}
\usepackage{graphicx}
% Same figure search paths as paper.tex (latexmk from Paper/ or repo root).
\graphicspath{{figures/}{Paper/figures/}}
\usepackage{booktabs}
\usepackage{tabularx}
\usepackage{float}

\begin{document}

\title{Supplementary Material: Hierarchical Transformer Preconditioning for Interactive Physics Simulation}

\author{Carl Osborne}
\affiliation{%
  \institution{MIT CSAIL}
  \city{Cambridge}
  \country{USA}}
\email{osbo@mit.edu}

\author{Minghao Guo}
\affiliation{%
  \institution{MIT CSAIL}
  \city{Cambridge}
  \country{USA}}
\email{guomh2014@gmail.com}

\author{Crystal Owens}
\affiliation{%
  \institution{MIT CSAIL}
  \city{Cambridge}
  \country{USA}}
\email{crystalo@mit.edu}

\author{Wojciech Matusik}
\affiliation{%
  \institution{MIT CSAIL}
  \city{Cambridge}
  \country{USA}}
\email{wojciech@csail.mit.edu}

\renewcommand{\shortauthors}{Osborne et al.}

\maketitle
\thispagestyle{plain}

This document collects the implementation details, dataset construction,
per-scale performance numbers, full train$\,\times\,$eval generalization grid
behind Table~6, and the precision/apply-path discussion that did not fit the
main-paper page budget. Section numbering is independent of the main paper.

% ===========================================================================
\section{Experimental Setup --- Full Details}
\label{supp:experimental-setup}
% ===========================================================================

\paragraph{Hardware.}
All GPU experiments run under a batch scheduler on a shared institutional GPU
cluster. Each job allocates one NVIDIA H200 (140\,GB HBM3), eight Intel Xeon
Platinum~8580 host cores, and 32\,GiB host DRAM alongside the device (partial-node
slice on dual-socket nodes with eight GPUs per node). CPU baselines use the same
eight host cores.

\paragraph{Software stack.}
GPU code is built with the CUDA~12 toolchain and a PyTorch \texttt{2.6.x} build
from a fixed Conda environment, using \verb|torch.compile| for graph capture. CPU
baselines use Eigen, SciPy, and PyAMG. Sparse matrix-vector products on the GPU use
the CSR layout produced by the dataset generator (Sec.~\ref{supp:dataset}). PCG
timing uses single-graph CUDA Graph replay for methods that admit it
(unpreconditioned CG, Jacobi, AMGX SPAI, neural SPAI, ours); IC- and AMG-class methods
are timed per launch since their sequential triangular solves and V-cycle synchronization
preclude single-graph capture.

\paragraph{Default model configuration.}
Unless noted, our model uses $d\!=\!128$, $n_l\!=\!3$, $L\!=\!128$,
$p_{\mathrm{diag}}\!=\!1$, $p_{\mathrm{off}}\!=\!4$ (so $L_s\!=\!32$),
$n_{\mathrm{gcn}}\!=\!2$, $h\!=\!8$ attention heads, highways enabled
(\textsf{d128\_L3\_hw} in figures). This single checkpoint is reused at every $N$
in the main performance table. Sec.~\ref{supp:architecture} expands the per-stage
shapes and Sec.~\ref{supp:training} the optimizer and probe details.

\paragraph{Baseline tuning.}
GPU IC (\textsc{multicolor\_dilu}) and GPU AMG settings follow AMGX vendor
defaults. At $N\!=\!8\,192$ we additionally swept the nearest neighboring AMGX
hyperparameter configurations (smoother type, coarsening strategy, maximum levels)
and verified that none meaningfully reduces total time relative to the default.
CPU PyAMG uses its default classical AMG cycle. AMGX SPAI is included as the
sparse-approximate-inverse data point; we keep its vendor defaults because the
neural SPAI baseline whose public implementation does not currently support our
problem class (main paper, footnote in \S7.1) would be the natural learned
comparison, not AMGX SPAI's hand-tuned variants.

\paragraph{Convergence criterion.}
All reported solve times and iteration counts are to a relative residual tolerance
of $\|\mathbf{r}_k\|_2 / \|\mathbf{r}_0\|_2 \!\le\! 10^{-8}$. This is two to three
orders of magnitude tighter than the $\sim\!10^{-3}$ accuracy typical of
graphics-grade pressure projection. We chose the tighter tolerance so per-method
comparisons reflect preconditioner quality rather than early termination; at
$10^{-3}$ every method finishes in fewer iterations, but the relative ordering and
ratios we report are preserved.

\paragraph{Precision.}
PCG scalar accumulators (dot products, residual norms, step sizes) use float64;
preconditioner weights and the apply path use float32. Sec.~\ref{supp:precision}
discusses why this split is sufficient on stiff systems at our target tolerance
and where each component sits within the apply-path memory budget.

% ===========================================================================
\section{Network Architecture Details}
\label{supp:architecture}
% ===========================================================================

This section expands the four-stage pipeline of main-paper~\S4 with the exact
tensor shapes and module-level choices needed to reproduce the network.

\paragraph{Encoder (Sec.~4.1).}
The per-node feature vector concatenates the simulator-exposed scalar fields
(density, pressure, geometric position, boundary indicators) with a broadcast
global context of dimension $d_{\mathrm{glob}}\!=\!12$ summarizing per-frame
statistics of the assembled system. A two-layer MLP with GELU activations lifts
this to width~$d$. The encoder then applies $n_{\mathrm{gcn}}\!=\!2$ residual
graph-convolutional layers~\cite{kipf2017semi} that use $A$ itself (normalized by
$\mathrm{diag}(A)$) as the message-passing weight. The encoder is the only stage
that touches individual edges; downstream stages consume only the per-node
embedding tensor of shape $(N, d)$.

\paragraph{Diagonal attention stack (Sec.~4.2).}
Encoder embeddings are reshaped from $(N, d)$ to $(K, L, d)$ and fed through $n_l$
transformer blocks with attention restricted to within-leaf token pairs (the
Swin-style local window of~\cite{Liu2021swin,vaswani2017attention} adapted to a
one-dimensional index range). Each block uses $h\!=\!8$ heads, head dimension
$d/h\!=\!16$, a GELU-activated FFN with $4d$ hidden width, pre-norm LayerNorm, and
residual connections. Attention logits carry a learned per-head bias produced by
a two-layer MLP from the four-dimensional edge descriptor
$(\Delta\mathbf{x}_{ij}, A_{ij})$.

\paragraph{Off-diagonal attention stack (Sec.~4.2).}
The same encoder embeddings are pooled along each tile's row- and column-strip
$\mathcal{I}_m, \mathcal{J}_m$ to obtain per-leaf coarse summaries, then
condensed along the in-strip axis to $L_s\!=\!L/p_{\mathrm{off}}\!=\!32$ tokens
per tile via uniform mean-pooling. Tile-grouped tokens then arrive at the
attention stack with shape $(M_{\mathcal{H}}, L_s, d)$, independent of the
physical tile size $S_mL$, and are processed by $n_l$ transformer blocks
identical in form to the diagonal stack (same head count, FFN width,
normalization). Edge biases for each in-tile token pair are computed from the
mean of $(\Delta\mathbf{x}_{ij}, A_{ij})$ over all node pairs spanning the
corresponding sub-strips.

\paragraph{Highway buffers (Sec.~4.3).}
After every attention sublayer in either stack, block-token embeddings are
scatter-added into per-layer row, column, and global buffers
$\mathbf{r}_{\mathrm{hw}}, \mathbf{c}_{\mathrm{hw}}\!\in\!\mathbb{R}^{B\times N\times d}$
and $\mathbf{g}_{\mathrm{hw}}\!\in\!\mathbb{R}^{B\times d}$ (off-diagonal tile
tokens are first repeat-interleaved back to full $L$-leaf resolution so each tile
contributes uniformly across its $S$ leaves). Before the FFN sublayer, each
token's row, column, and global highway slices are concatenated with its own
$d$-dim embedding and the resulting $4d$-wide vector is fed through the FFN input
projection. The four-channel mix (2D local + 1D row + 1D column + 0D broadcast)
is repeated independently in every transformer block; the buffers themselves are
not residual across blocks.

\paragraph{Decoder heads (Sec.~4.4).}
Three lightweight heads project token embeddings to the factor tensors that the
apply path consumes. The leaf head is a two-layer MLP per diagonal-stream token
followed by a reshape into $F_k\!\in\!\mathbb{R}^{L\times L}$. The two
off-diagonal heads are single linear layers producing
$U_m, V_m\!\in\!\mathbb{R}^{L_s\times L_s}$ from the off-diagonal-stream tokens
($L_s$ tokens per tile, one head emits $U_m$, the other $V_m$). The two node
heads are single linear layers producing the bridge matrices
$\tilde U_k, \tilde V_k\!\in\!\mathbb{R}^{L\times L_s}$ from the diagonal-stream
per-node embeddings. A final scalar gate produces the Jacobi-residual weight
$\lambda_i$.

\paragraph{Apply-path tensor layout.}
The decoder outputs are concatenated into a single packed tensor of width
$P\!=\!KL^2 + M_{\mathcal{H}} L_s^2 + 2NL_s + N$ with strides aligned to the
$\mathcal{H}$-matrix partition. With the weak-admissibility $\mathcal{H}$-matrix partition at
admissibility parameter $\eta\!=\!1$, the number of \emph{unique} off-diagonal
tiles satisfies $M_{\mathcal{H}}\!=\!K\!-\!1$ (geometric sum
$K/2 + K/4 + \cdots + 1$ over the strict upper triangle); the symmetric lower
triangle reuses the same $B_m$ via the transposed apply
$\mathbf{t}^{\mathrm{c}}_m\!=\!B_m^\top\mathbf{s}^{\mathrm{r}}_m$ from the
main-paper Sec.~5 equations. Concrete factor-tensor sizes at the scales of the main paper's
performance table (main paper Table~4) are listed in Sec.~\ref{supp:precision}.

\paragraph{Explicit off-diagonal apply equations (main paper Sec.~5).}
For leaf residual $\mathbf{r}_k\!\in\!\mathbb{R}^{L}$ and tile leaf-ranges
$\mathcal{R}_m,\mathcal{C}_m$, the off-diagonal contribution follows the same
FMM-style chain used in the main text:
\begin{align}
  \hat{\mathbf{u}}_k &= \tilde U_k^\top\mathbf{r}_k,\qquad
  \hat{\mathbf{v}}_k = \tilde V_k^\top\mathbf{r}_k && \text{(restriction)} \\
  \mathbf{s}^{\mathrm{r}}_m &= \sum_{k\in\mathcal{R}_m}\hat{\mathbf{u}}_k,\qquad
  \mathbf{s}^{\mathrm{c}}_m = \sum_{k\in\mathcal{C}_m}\hat{\mathbf{v}}_k
  && \text{(strip aggregation)} \\
  \mathbf{t}^{\mathrm{c}}_m &= B_m^\top\mathbf{s}^{\mathrm{r}}_m,\qquad
  \mathbf{t}^{\mathrm{r}}_m = B_m\mathbf{s}^{\mathrm{c}}_m && \text{(coarse coupling)} \\
  \Delta\mathbf{y}_k &= \tilde U_k\,{\textstyle\sum_{m:k\in\mathcal{R}_m}\!\mathbf{t}^{\mathrm{r}}_m}
                    +  \tilde V_k\,{\textstyle\sum_{m:k\in\mathcal{C}_m}\!\mathbf{t}^{\mathrm{c}}_m}
  && \text{(prolongation).}
\end{align}
The stage-wise shape progression for one tile of span $S_mL$ is
$S_mL \rightarrow S_mL_s \rightarrow L_s \rightarrow L_s \rightarrow S_mL_s \rightarrow S_mL$.
In implementation this is four batched GEMMs with shapes
$(K,L,L_s)$, $(M_{\mathcal{H}},L_s,L_s)$, $(K,L,L_s)$ (restriction, coupling,
prolongation; two directional bridge passes share the same launch shape), plus two
partition-indexed scatter-adds for strip aggregation and redistribution.

% ===========================================================================
\section{Training Procedure}
\label{supp:training}
% ===========================================================================

\paragraph{Optimizer and schedule.}
We train with AdamW (PyTorch defaults for $\beta_1,\beta_2,\epsilon$,
weight decay $10^{-4}$) at initial learning rate $2\!\times\!10^{-4}$. Learning
rate is reduced on plateau with \texttt{ReduceLROnPlateau} (factor $0.5$,
patience $5$ log steps, relative threshold $5\!\times\!10^{-3}$, minimum
$\max(\mathrm{lr}\!\times\!10^{-3}, 10^{-6})$). Gradients are globally clipped to
$\ell_2$ norm $1$ before each AdamW step.

\paragraph{Auto-stop.}
Training proceeds for at most $10^5$ optimizer steps but is terminated early once
the LR scheduler reaches \texttt{min\_lr} \emph{and} the cosine-Hutchinson loss
has failed to improve by the same $5\!\times\!10^{-3}$ relative threshold over
$10$ consecutive log steps (twice the LR-scheduler patience). At our default
configuration this fires at roughly $24\,300$ steps (main paper, \S7.3).

\paragraph{Probe vectors.}
At each step we draw a batch of $K_z\!=\!\max(64, \lceil\sqrt{N}\rceil)$ probe
vectors $\mathbf{Z}\!\sim\!\mathcal{N}(0, I)$ and apply two damped-Jacobi
smoothing sweeps with $\omega\!=\!0.6$ (main paper, Eq.~8) to redistribute probe
energy toward lower spatial frequencies. Probes are detached after smoothing, so
no gradient flows back through the smoother. The constant $64$ floor on $K_z$
keeps gradient noise bounded at the smallest scales; the $\sqrt{N}$ growth keeps
the per-step gradient signal-to-noise ratio approximately constant as $N$ grows.

\paragraph{Gradient accumulation.}
Each optimizer step aggregates gradients over four random cached training
contexts (graph, $A$, masks, padded sizes, smoothed probes). Contexts are
precomputed once and cached on disk so the per-step cost is dominated by the
forward/backward through the network rather than dataset assembly.

\paragraph{$\mathcal{H}$-matrix partition.}
The weak-admissibility partition is constructed once per scale at training start
with admissibility parameter $\eta\!=\!1$ and the leaf count $K\!=\!N/L$
determined by the scale. The partition is keyed to $N$ and reused unchanged on
every test frame at that scale; no part of the partition depends on $A$ or the
right-hand side.

\paragraph{Wall-clock budget.}
End-to-end training of the default configuration is $\sim\!16$\,min on one
H200 at $N\!=\!8\,192$, with the model overtaking GPU Jacobi at step
$\sim\!2\,000$ ($\sim\!1.3$\,min) and dropping under $200$ PCG iterations by
step $\sim\!12\,000$ ($\sim\!8$\,min). The training profile is plotted in main
paper Fig.~4.

% ===========================================================================
\section{Multiphase Poisson Benchmark Generation}
\label{supp:dataset}
% ===========================================================================

This appendix gives the precise procedure for generating each frame of the
multiphase Poisson benchmark used throughout the main paper.

\paragraph{Grid and ordering.}
Each frame targets $N$ degrees of freedom on a 2D structured grid of dimensions
$W\!\times\!H$ with $W\!\cdot\!H\!\ge\!N$ and $W,\,H$ chosen as close to square as
possible. All $W\!\cdot\!H$ cells are sorted by Morton (Z-order) code and
truncated to the first $N$ cells, giving a contiguous Morton-ordered index set.
Edges and density values follow the same ordering. We use a structured grid
(rather than a particle cloud) so that the assembled $A$ has the canonical
5-point Laplacian sparsity pattern, isolating the effect of the heterogeneous
coefficient field on conditioning.

\paragraph{Density field.}
Per frame the heavy density $\rho_{\text{heavy}}$ is drawn log-uniformly from
$[5, 100]$ with $\rho_{\text{light}}\!=\!1$. We then sample $n_b\!\sim\!\mathrm{Uniform}\{1,2,3\}$
\emph{barriers}; each barrier is independently
\begin{enumerate}
\item assigned an orientation (vertical or horizontal, equiprobable);
\item given a center coordinate drawn uniformly from $[0.2, 0.8]$ along the cross
axis, in normalized grid coordinates;
\item given a thickness drawn uniformly from $[0.05, 0.20]$;
\item given a gap topology drawn uniformly from
$\{\text{top},$ $\text{bottom},$ $\text{middle\_hole},$ $\text{closed}\}$.
\end{enumerate}
A cell is heavy iff it lies in the heavy region of \emph{any} barrier, so
multiple barriers can overlap to form cross- or L-shaped inclusions. Each cell's
density is finally multiplied by $1\!+\!\mathcal{N}(0, 0.05^2)$ for fine-grain
symmetry breaking.

\paragraph{Operator assembly.}
$A$ is the standard 5-point pressure-Poisson Laplacian with harmonic-mean face
conductance $w_{ij}\!=\!2\rho_i\rho_j/(\rho_i\!+\!\rho_j)$, evaluated on
cell-cell faces. Boundary cells use zero-flux (Neumann) boundary conditions, as
is standard for incompressible pressure-projection in graphics-grade fluid
simulators. We do \emph{not} apply a zero-mean constraint to the resulting
null-space mode; CG handles it implicitly when the right-hand side is consistent.

\paragraph{Right-hand side.}
For each frame we draw $\mathbf{b}\!\sim\!\mathcal{N}(0, I)$ projected onto the
orthogonal complement of the constant vector ($\mathbf{1}^\top\mathbf{b}\!=\!0$
to ensure consistency with the Neumann null-space). This is a worst-case
right-hand-side distribution from a preconditioner's perspective: it weights all
spatial frequencies equally, including the low ones that are hardest for local
preconditioners.

\paragraph{Per-scale dataset sizes.}
For each of five scales, spanning $N=1\,024$ to $N=16\,384$, we generate
$100$ training frames and $20$ test frames with disjoint seeds.
Training and test split the same generator distribution.

% ===========================================================================
\section{Per-frame Iteration-count Variability}
\label{supp:full_perf_table}
% ===========================================================================

The consolidated per-scale times and mean iteration counts have moved to the
main paper, Table~4. This section reports the across-frame variability
($\pm 1\sigma$ over the same $20$ test frames per scale) that the main table
omits to fit the column budget.

\begin{table}[H]
\centering
\caption{Per-frame mean$\pm$std PCG iteration counts on the multiphase Poisson
benchmark ($\mathrm{rtol}\!=\!10^{-8}$, $20$ frames per scale). Bold row marks
the proposed method.}
\label{tab:full_perf_table}
\footnotesize\setlength{\tabcolsep}{3pt}
\resizebox{\columnwidth}{!}{%
\begin{tabular}{@{}l ccccc@{}}
\toprule
Method & $N\!=\!1\,024$ & $N\!=\!2\,048$ & $N\!=\!4\,096$ & $N\!=\!8\,192$ & $N\!=\!16\,384$ \\
\midrule
Unprec.~CG (GPU)             & $497\!\pm\!144$ & $650\!\pm\!240$ & $1153\!\pm\!434$ & $1765\!\pm\!1744$ & $2103\!\pm\!1113$ \\
Jacobi (GPU)                 & $325\!\pm\!83$  & $429\!\pm\!112$ & $839\!\pm\!476$  & $968\!\pm\!261$   & $1543\!\pm\!1137$ \\
IC / DILU (GPU)              & $11\!\pm\!1$    & $15\!\pm\!1$    & $22\!\pm\!4$     & $30\!\pm\!5$      & $40\!\pm\!4$ \\
AMG / AMGX (GPU)             & $1\!\pm\!0$     & $1\!\pm\!0$     & $1\!\pm\!1$      & $2\!\pm\!0$       & $3\!\pm\!0$ \\
Neural SPAI (GPU)~\cite{Yang2025sparse} & $118\!\pm\!6$   & $167\!\pm\!8$   & $246\!\pm\!41$   & $338\!\pm\!24$    & $496\!\pm\!107$ \\
IC (CPU)                     & $59\!\pm\!18$   & $96\!\pm\!23$   & $113\!\pm\!31$   & $170\!\pm\!47$    & $254\!\pm\!61$ \\
AMG (CPU)                    & $5\!\pm\!6$     & $9\!\pm\!6$     & $5\!\pm\!7$      & $7\!\pm\!8$       & $10\!\pm\!8$ \\
\textbf{Ours (GPU)}          & $\mathbf{47\!\pm\!9}$ & $\mathbf{66\!\pm\!16}$ & $\mathbf{80\!\pm\!24}$ & $\mathbf{168\!\pm\!26}$ & $\mathbf{394\!\pm\!68}$ \\
\bottomrule
\end{tabular}
}
\end{table}

\noindent
The neural SPAI baseline is re-trained per scale (one network per $N$) using
the SAI loss of~\cite{Yang2025sparse} on the same training distribution as
ours; the row reports mean$\pm$std across the same per-scale test-frame
evaluation as the other methods.

% ===========================================================================
\section{Generalization Robustness}
\label{supp:generalization}
% ===========================================================================

Table~6 in the main paper reports four cells of a wider train$\,\times\,$eval
grid that probes within-family robustness at $N\!=\!4\,096$.
Table~\ref{supp-tab:generalization} reports the full grid for \emph{our}
method, adding both the in-distribution row (\emph{Full} training,
evaluated on closed-only and high-contrast subsets) and a fourth,
compositional training distribution that excludes closed barriers
\emph{and} restricts contrast to $\rho_{\text{heavy}}\!\in\![5,25]$.

\begin{table}[H]
\centering
\caption{Within-family generalization grid for the proposed method at
$N\!=\!4\,096$ ($\mathrm{rtol}\!=\!10^{-8}$, $20$ frames per cell). Each cell
reports mean$\pm$std PCG iterations; dashes mark cells that are
in-distribution for the corresponding training set (so the entry would
duplicate the leftmost column). The fourth training row is a compositional
distribution that excludes closed barriers \emph{and} restricts contrast to
$\rho_{\text{heavy}}\!\in\![5,25]$; the rightmost column evaluates it on the
joint shift (closed barriers $+$ high contrast).}
\label{supp-tab:generalization}
\footnotesize\setlength{\tabcolsep}{4pt}
\begin{tabular}{@{}l cccc@{}}
\toprule
& \multicolumn{4}{c}{Eval distribution} \\
\cmidrule(lr){2-5}
Train distribution & Full (id) & Closed only & High contrast & Closed $+$ high \\
\midrule
Full                          & $82\!\pm\!28$  & ---            & ---             & ---             \\
Excl.\ closed barriers        & $78\!\pm\!19$  & $68\!\pm\!16$  & ---             & ---             \\
Low contrast                  & $78\!\pm\!26$  & ---            & $142\!\pm\!126$ & ---             \\
Excl.\ closed $+$ low $\rho$  & $95\!\pm\!29$  & $89\!\pm\!20$  & $153\!\pm\!97$  & $147\!\pm\!102$ \\
\midrule
Mean total solve (ms)         & $8.2$--$9.5$   & $7.4$--$9.0$   & $13.1$--$13.9$  & $13.5$          \\
$\Delta_{\text{OOD}}$ (iters) & $1.00$ (def.)  & $0.87$--$0.94$ & $1.82$, $1.61$  & $1.55$          \\
\bottomrule
\end{tabular}
\end{table}

\noindent
$\Delta_{\text{OOD}}$ is the ratio of iterations in the cell to the
in-distribution cell of the same training row (lower is better). Row~1
(\emph{Full}) is included so the in-distribution operating point is on the
same page as the OOD numbers; we omit its trivial OOD columns.

The grid shows that topology shift is inexpensive
($\Delta_{\text{OOD}}\!=\!0.87$--$0.94$), while contrast shift is the dominant
OOD cost ($\Delta_{\text{OOD}}\!=\!1.55$--$1.82$). Even in the compositional
shift cell (closed $+$ high contrast), the model remains at $1.9\times$
Jacobi-relative speedup.

% ===========================================================================
\section{Precision and Hardware Efficiency}
\label{supp:precision}
% ===========================================================================

This section expands the precision and apply-path arguments referenced from main
paper~\S5 and~\S7.1.

\paragraph{Mixed precision split and its motivation.}
The apply path consists of dense batched GEMMs of shapes $(K, L, L)$,
$(M_{\mathcal{H}}, L_s, L_s)$, and $(K, L, L_s)$ (main paper~\S5). At
$L\!=\!128, L_s\!=\!32$ each individual matmul has condition number bounded by
the singular-value spread of its factor (typically $\le\!10^3$ in our trained
models), well within float32's $\sim\!10^7$ representable range. PCG's scalar
accumulators, by contrast, run over the whole residual vector and accumulate
$O(N)$ terms per iteration; on stiff multiphase systems we observed residual
norms drift by $1$--$2$ orders of magnitude over a few hundred iterations when
those accumulators were held at float32, which can cause spurious early
termination at $\mathrm{rtol}\!=\!10^{-8}$. Holding only the scalar
accumulators (dot products, residual norms, step sizes) at float64 eliminates
that drift without paying float64's $2\!\times$ memory/throughput penalty on
the bulk GEMMs. This is the same precision split used in CG implementations in
cuSPARSE and AMGX.

\paragraph{Factor-tensor memory footprint.}
The packed factor tensor of width $P\!=\!KL^2 + M_{\mathcal{H}} L_s^2 + 2NL_s + N$
(main paper~\S4.4) determines the apply-path memory budget. With $L\!=\!128$,
$L_s\!=\!32$, and $M_{\mathcal{H}}\!=\!K\!-\!1$ at $\eta\!=\!1$
weak admissibility, Table~\ref{tab:supp_memory} lists the absolute numbers at
the scales in Table~\ref{tab:full_perf_table}.

\begin{table}[H]
\centering
\caption{Factor-tensor breakdown for the default configuration
($L\!=\!128, L_s\!=\!32, p_{\mathrm{off}}\!=\!4$). $K\!=\!N/L$ is the leaf
count; $M_{\mathcal{H}}\!=\!K\!-\!1$ is the unique off-diagonal tile count
under weak admissibility ($\eta\!=\!1$); $P$ is the total packed width in
float32 elements; ``MB'' is the resulting on-device footprint.}
\label{tab:supp_memory}
\footnotesize\setlength{\tabcolsep}{4pt}
\begin{tabular}{@{}r rrr rr@{}}
\toprule
$N$ & $K$ & $M_{\mathcal{H}}$ & $KL^2$ & $P$ & MB \\
\midrule
$1\,024$  & $8$            & $7$   & $0.131$\,M & $0.20$\,M & $0.82$ \\
$2\,048$  & $16$           & $15$  & $0.262$\,M & $0.41$\,M & $1.64$ \\
$4\,096$  & $32$           & $31$  & $0.524$\,M & $0.82$\,M & $3.29$ \\
$8\,192$  & $64$           & $63$  & $1.049$\,M & $1.65$\,M & $6.58$ \\
$16\,384$ & $128$          & $127$ & $2.097$\,M & $3.29$\,M & $13.2$ \\
\bottomrule
\end{tabular}
\end{table}

\noindent
The factor tensor scales linearly in $N$ at fixed $L$ and stays below
$10$\,MB through $N\!=\!8\,192$; at $N\!=\!16\,384$ it reaches
$13.2$\,MB and still fits comfortably in a single H200's HBM. The dominant term
at every scale is $KL^2$ (the dense diagonal
leaves), not $M_{\mathcal{H}} L_s^2$: distant tiles are compressed so
aggressively that the entire off-diagonal contribution costs less than the
diagonal even though it covers $1\!-\!1/K$ of the matrix.

\paragraph{Apply-path kernel breakdown.}
Main paper Table~3 reports the kernel-family split at $N\!=\!8\,192$: CUTLASS
Tensor-Op GEMMs ($31\%$) plus CUTLASS fused attention ($14\%$) account for
$\sim\!45\%$ of device time; the remaining $\sim\!55\%$ is elementwise
operations, layout reshapes, and small bookkeeping kernels.

\paragraph{What would have to change for tighter tolerance.}
The float32 apply path supports $\mathrm{rtol}\!\le\!10^{-8}$ across all scales
we evaluate. For graphics applications this is two to three orders of
magnitude tighter than typical pressure-projection tolerances and is therefore
sufficient. For scientific applications requiring $\mathrm{rtol}\!\le\!10^{-10}$
or stricter, the apply path would either need a full float64 pass (doubling
device-memory and halving Tensor-Core throughput) or an outer iterative
refinement loop that uses the float32 apply as an inner preconditioner. We did
not implement either since they fall outside the regime we target.

% ===========================================================================
\section{Additional Figures and Tables Referenced from the Main Paper}
\label{supp:floats}
% ===========================================================================

This section provides optional figures and detailed-breakdown tables for
readers who want additional clarity on the method and results. Main-paper
cross-references resolve to the \emph{Figure}/\emph{Table} number shown next to
each caption below.

% --- partition + highways graphic (was Fig. 2 in earlier drafts) ---
\begin{figure}[H]
  \centering
  \begin{minipage}[t]{0.49\linewidth}\centering
    \includegraphics[width=\linewidth]{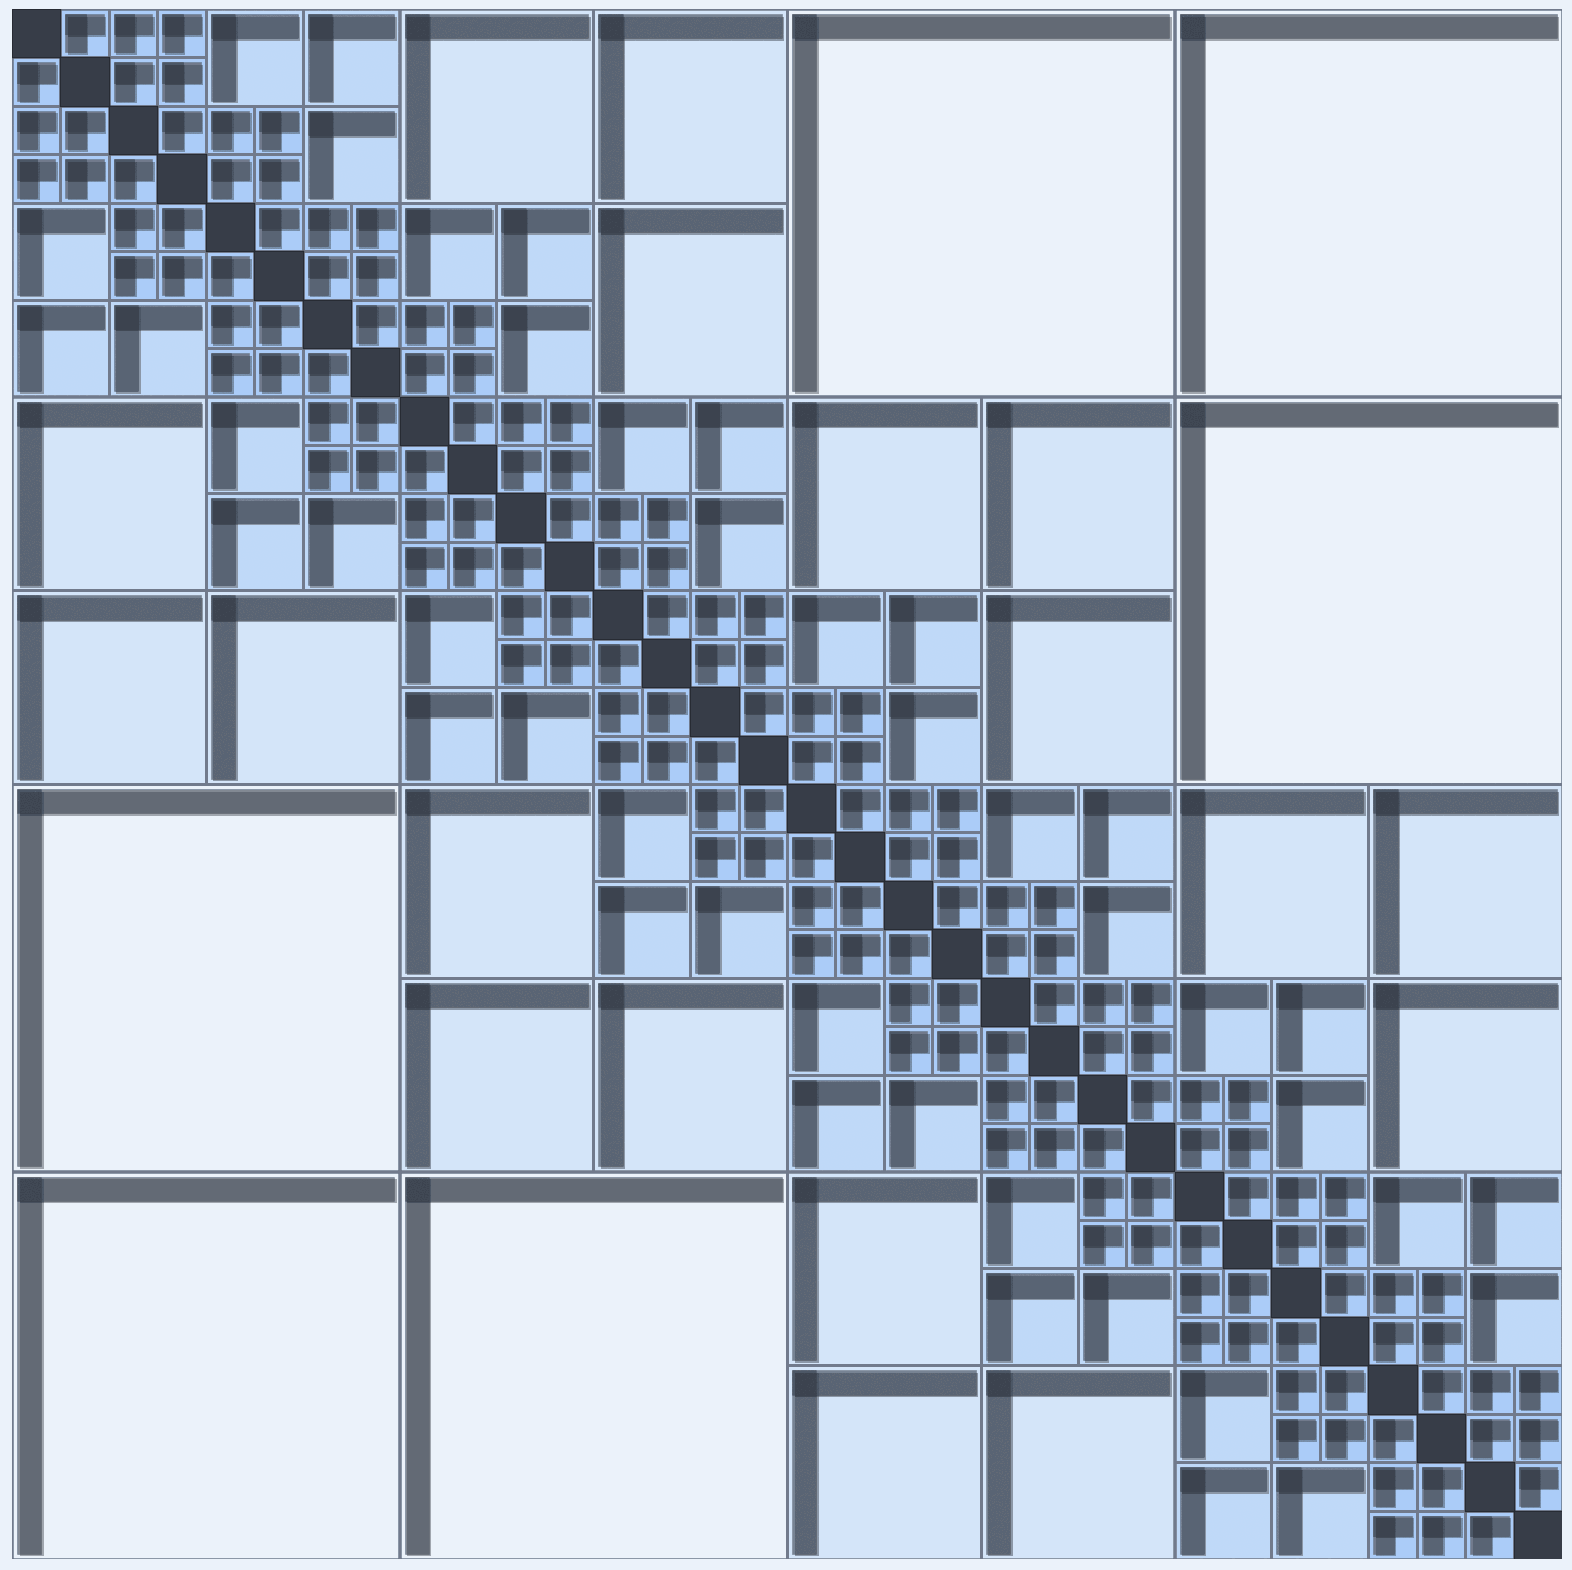}\\
    \small (a) $\mathcal{H}$-matrix partition.
  \end{minipage}\hfill
  \begin{minipage}[t]{0.49\linewidth}\centering
    \includegraphics[width=\linewidth]{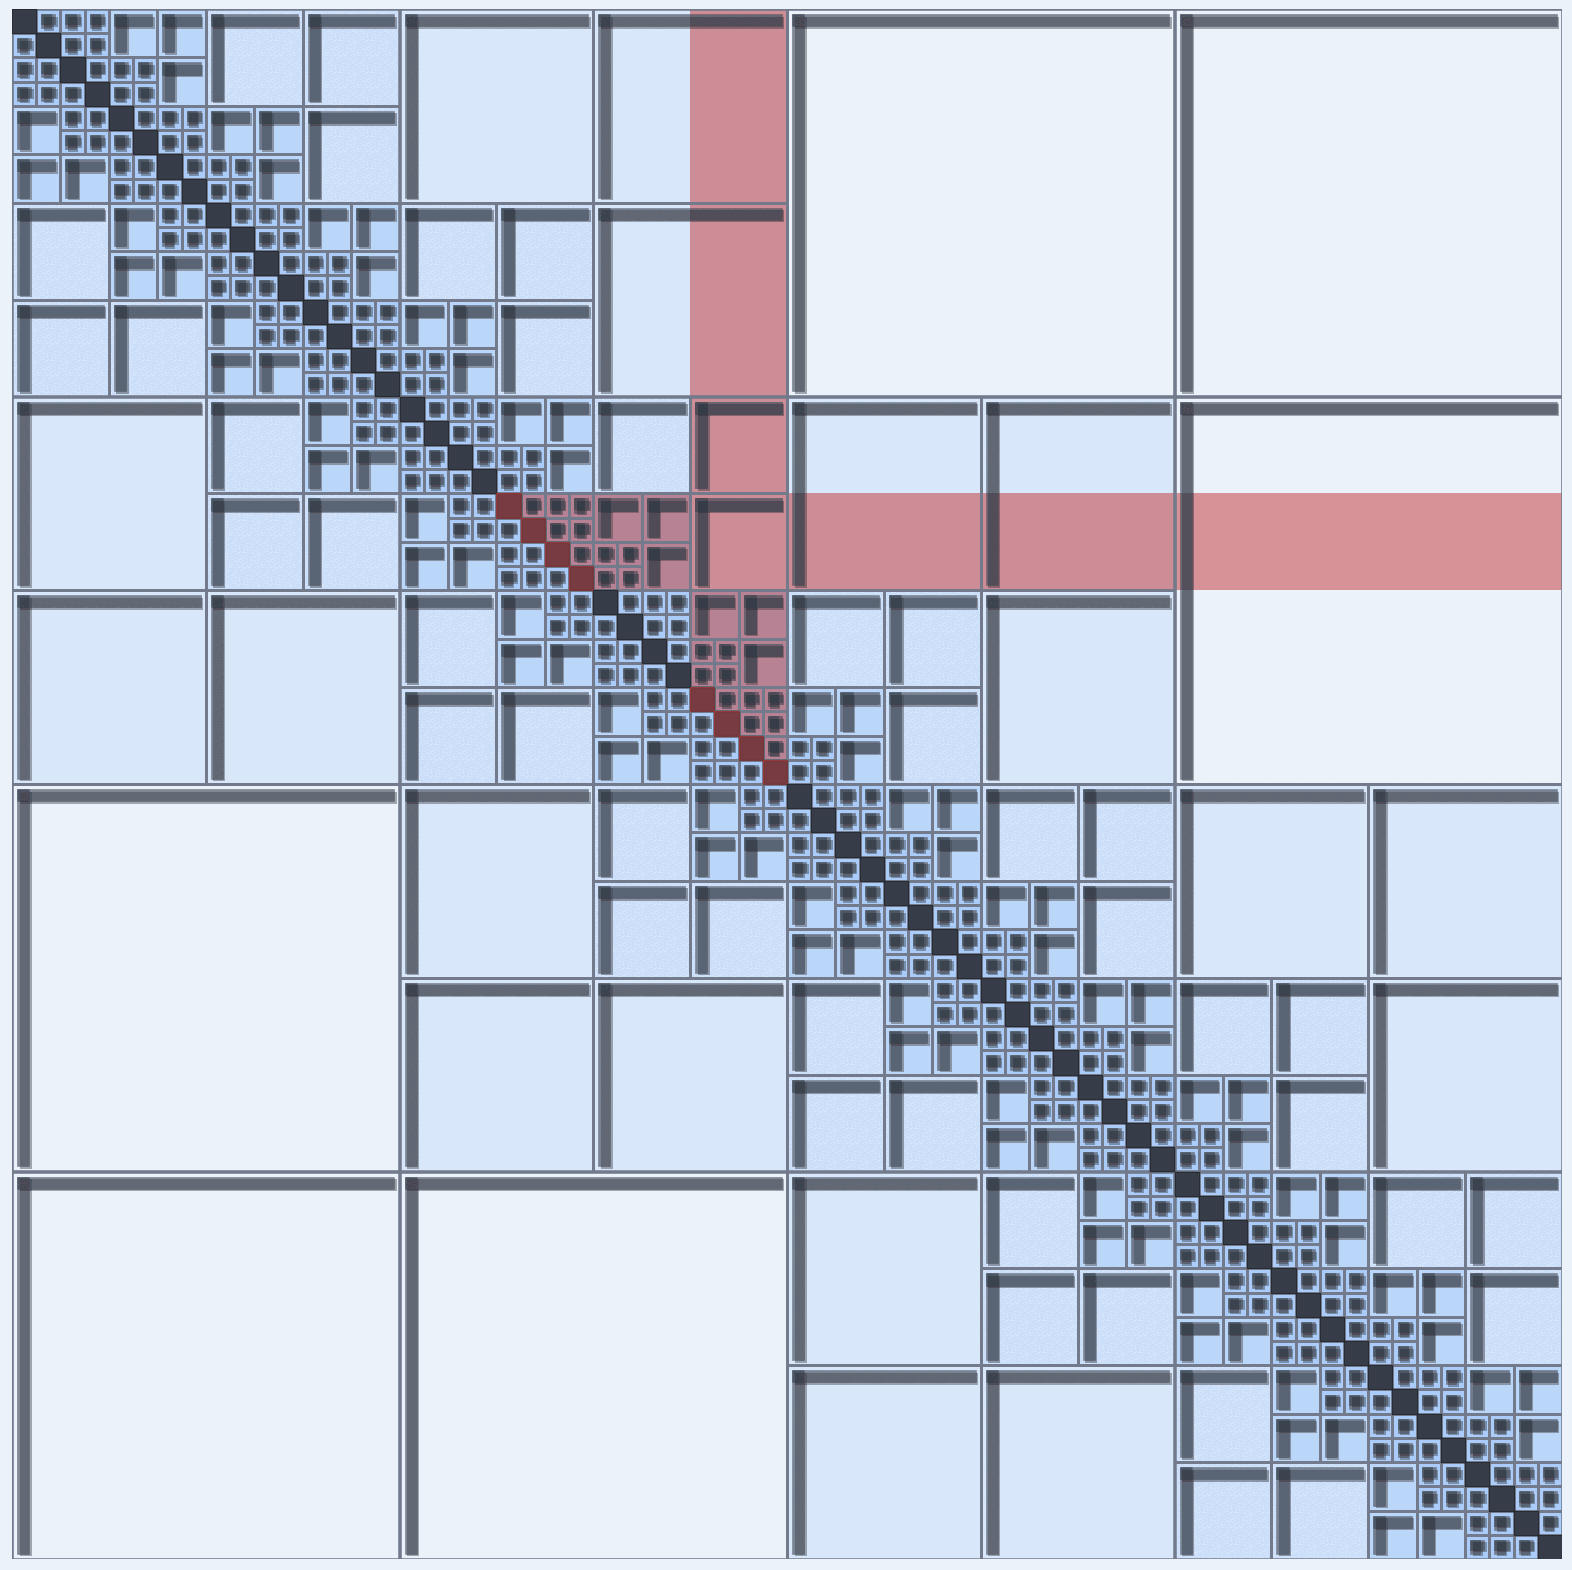}\\
    \small (b) Highway channels.
  \end{minipage}
  \caption{\emph{Left:} weak-admissibility $\mathcal{H}$-matrix partition. Dense
    diagonal leaves along the main diagonal; admissible off-diagonal tiles
    double in size with separation. \emph{Right:} per-layer highway channels.
    One red overlay marks the row- and column-index sets of a representative
    off-diagonal tile; this tile contributes scatter-adds to those strips and
    to a single global token --- four communication channels of dimensions
    2D / 1D / 1D / 0D per layer.}
  \label{supp-fig:partition-and-highways}
\end{figure}

% --- assembled-matrix panel (panel (a) of the earlier combined figure;
%     the rank-fraction audit (panel (b)) has been promoted to the main
%     paper's figure-only pages and is referenced from there). ---
\begin{figure}[H]
  \centering
  \includegraphics[width=0.85\linewidth]{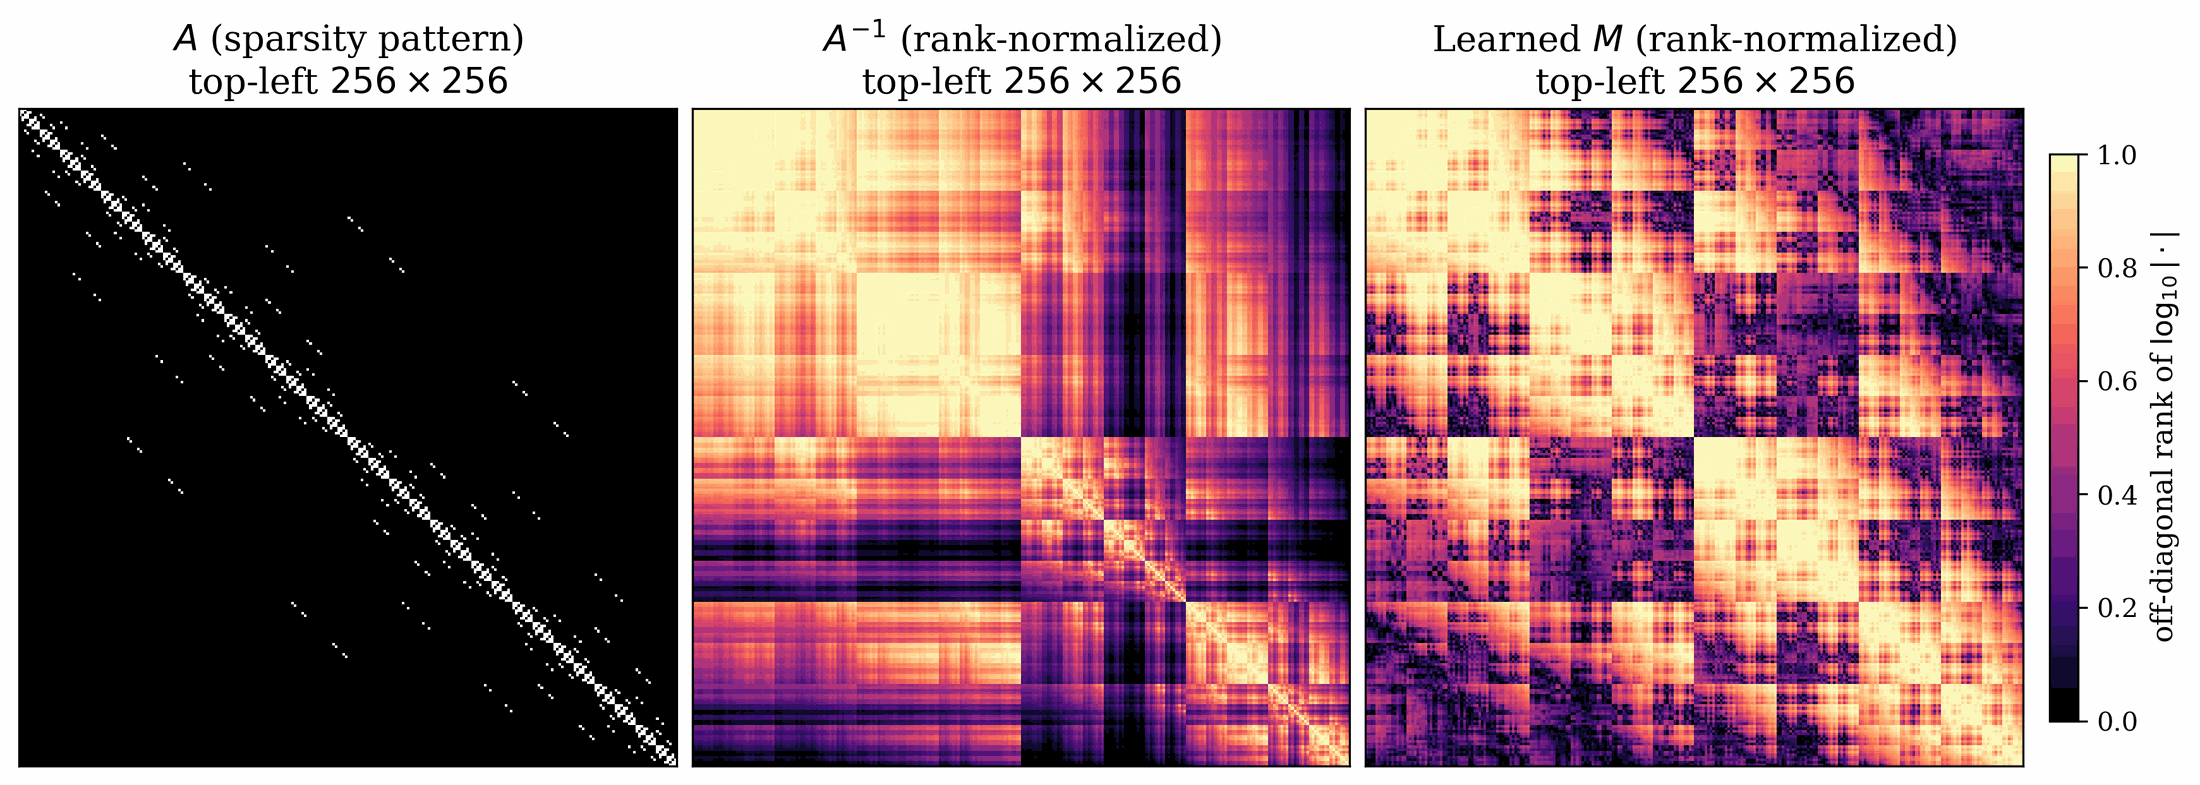}
  \caption{The sparse operator $A$, its dense inverse $A^{-1}$, and the
    assembled learned $M\!\approx\!A^{-1}$ (top-left $256\!\times\!256$)
    on a multiphase pressure-Poisson frame, on a shared rank-normalized
    color scale. All three share the weak-admissibility block-and-tile
    pattern: full-rank diagonal blocks plus off-diagonal tiles whose
    magnitude decays with separation. This pattern is exactly the prior
    quantified by main paper Fig.~3.}
  \label{supp-fig:matrices}
\end{figure}

% --- benchmark frame (was Fig. 4 in earlier drafts) ---
\begin{figure}[H]
  \centering
  \includegraphics[width=\linewidth]{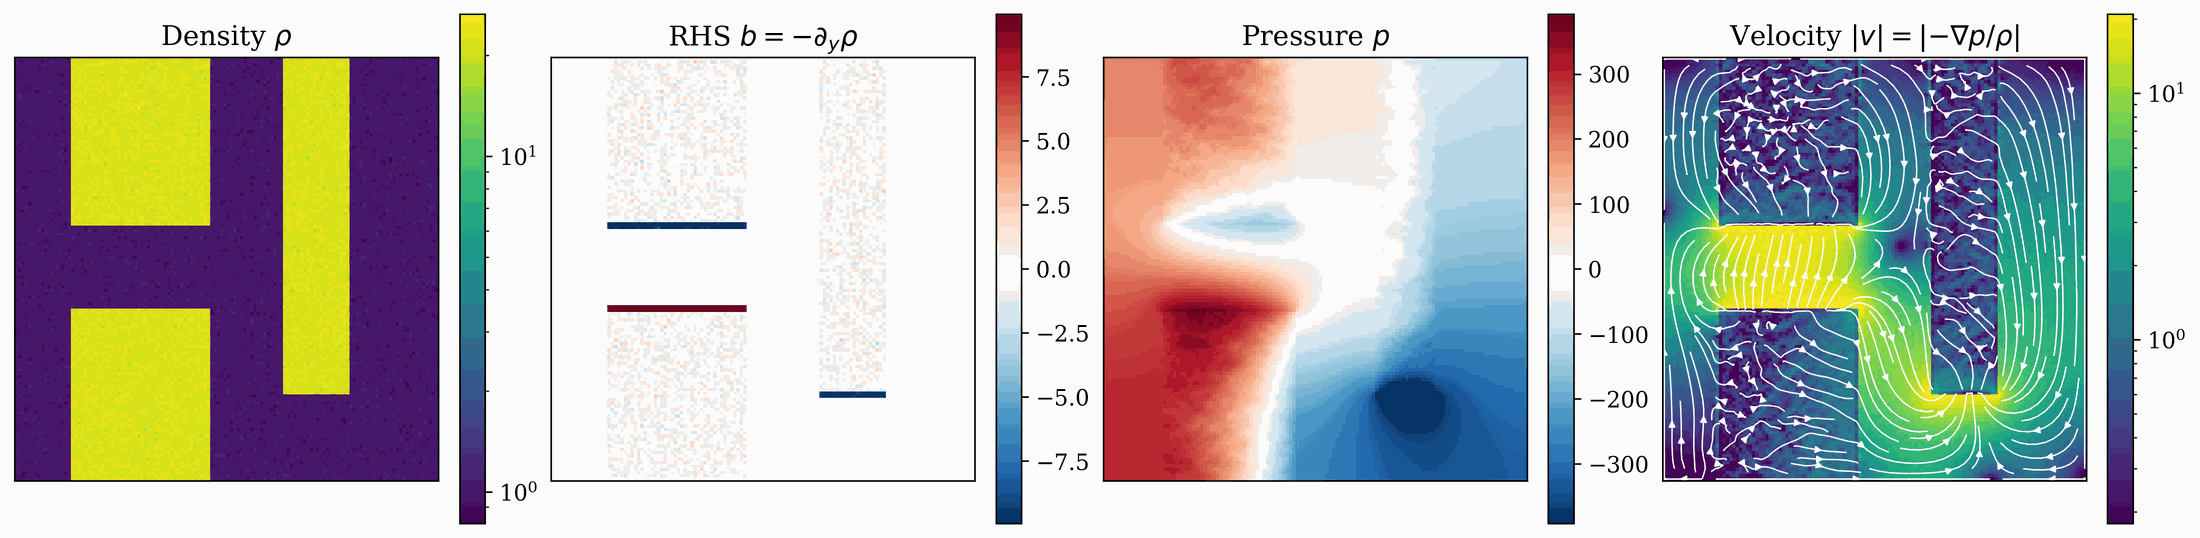}
  \caption{A representative frame from our multiphase pressure-Poisson
    benchmark at $N\!=\!16\,384$. \emph{Left:} heterogeneous density $\rho$ with
    $27\!\times$ contrast, separated by closed and partially-closed barriers
    (yellow). \emph{Middle:} buoyancy-driven right-hand side
    $b\!=\!-\partial_y\rho$, concentrated on horizontal density interfaces.
    \emph{Right:} recovered pressure $p$ with velocity $-\nabla p/\rho$
    overlaid.}
  \label{supp-fig:bench-frame}
\end{figure}

% --- hyperparameter ablation (main-paper Table 5 core rows; full grid here) ---
\begin{table}[H]
\centering
\caption{Hyperparameter ablations on multiphase Poisson ($\mathrm{rtol}\!=\!10^{-8}$,
$20$~frames per scale, neural preconditioner only). Train = wall-clock to
convergence; Infer.\ = preconditioner forward pass; Iters = mean PCG iters;
Total = inference $+$ PCG solve; $\Delta$ solve time = fractional change vs.\
the ``---'' row.}
\label{supp-tab:ablation}
\footnotesize\setlength{\tabcolsep}{3.5pt}
\begin{tabular}{@{}l rr rr r@{}}
\toprule
Configuration & Train & Infer. & Iters & Total & $\Delta$ solve \\
              & (min) & (ms)   &       & (ms)  & time \\
\midrule
\multicolumn{6}{l}{\emph{Width} (avg.\ $N\!\in\!\{2048,4096,8192\}$):}\\
$d{=}64,\;n_l{=}3$, hw     &  9.5 & 3.0 & 147 & 15.4 & $+28\%$  \\
$d{=}128,\;n_l{=}3$, hw    & 10.7 & 3.1 & 105 & 12.0 & ---      \\
$d{=}256,\;n_l{=}3$, hw    & 12.3 & 3.2 & 191 & 19.3 & $+61\%$  \\
\midrule
\multicolumn{6}{l}{\emph{Depth} ($N\!=\!8192$):}\\
$d{=}128,\;n_l{=}1$, hw    &  6.1 & 1.3 & 421 & 36.9 & $+106\%$ \\
$d{=}128,\;n_l{=}2$, hw    &  9.6 & 2.3 & 218 & 20.8 & $+16\%$  \\
$d{=}128,\;n_l{=}3$, hw    & 16.2 & 3.4 & 168 & 17.9 & ---      \\
\midrule
\multicolumn{6}{l}{\emph{Highways} ($N\!=\!2048$):}\\
$d{=}128,\;n_l{=}3$, hw    &  6.0 & 3.3 &  66 &  8.8 & ---      \\
$d{=}128,\;n_l{=}3$, no-hw &  4.8 & 2.2 & 149 & 13.8 & $+58\%$  \\
\bottomrule
\end{tabular}
\end{table}

% --- neural runtime components (supplementary; complements main Table~4) ---
\begin{table}[H]
\centering
\caption{Neural-method runtime components by scale: preconditioner inference
and PCG solve time (ms), plus total time and iterations aligned with the
main-paper performance table. Neural SPAI uses the re-trained-per-scale CUDA
apply path of~\cite{Yang2025sparse}.}
\label{supp-tab:neural_time_components}
\footnotesize\setlength{\tabcolsep}{5pt}
\begin{tabular}{@{}lcccc@{}}
\toprule
Scale $N$ & Infer. (ms) & Solve (ms) & Total (ms) & Iters \\
\midrule
\multicolumn{5}{@{}l}{\textit{Neural SPAI (GPU, CUDA apply)~\cite{Yang2025sparse}}}\\
$1\,024$  & 4.6  & 13.8 & 18.4 & 118 \\
$2\,048$  & 3.8  & 22.2 & 26.0 & 167 \\
$4\,096$  & 6.6  & 31.7 & 38.3 & 246 \\
$8\,192$  & 4.4  & 43.8 & 48.1 & 338 \\
$16\,384$ & 4.9  & 66.0 & 70.9 & 496 \\
\midrule
\multicolumn{5}{@{}l}{\textit{Ours (GPU)}}\\
$1\,024$  & 1.9  & 5.1  & 7.0  & 47  \\
$2\,048$  & 1.9  & 6.9  & 8.8  & 66  \\
$4\,096$  & 2.2  & 7.0  & 9.2  & 80  \\
$8\,192$  & 4.0  & 13.9 & 17.9 & 168 \\
$16\,384$ & 17.0 & 30.6 & 47.6 & 394 \\
\bottomrule
\end{tabular}
\end{table}

\bibliographystyle{ACM-Reference-Format}
\bibliography{references}

\end{document}
